# Supplementary material for: Sub-femtosecond wakefield injector and accelerator based on an undulating plasma bubble controlled by a laser phase
Source: arXiv:2103.13781 ancillary file (2021-04-25)
Supplement: Supplementary file 1 [file CEP_paper_Draft__Supplement.pdf]

# Sub-femtosecond wakefield injector and accelerator based on an undulating plasma bubble controlled by a laser phase

Jihoon Kim<sup>1</sup>, Tianhong Wang<sup>1</sup>, Vladimir Khudik<sup>1,2</sup>, and Gennady Shvets<sup>1</sup>

<sup>1</sup>*School of Applied and Engineering Physics, Cornell University, Ithaca, NY 14850, USA.*

<sup>2</sup>*Department of Physics and Institute for Fusion Studies,  
The University of Texas at Austin, Austin, TX 78712, USA.*

## I. DISCUSSION OF INJECTION CONDITION

In this section, we reproduce the parameter-free bubble equation following[1] for convenience, which is in turn used to calculate maximum transverse momentum that electrons can gain while passing through a relativistic bubble. Using this result, we derive our injection criterion. We show the Hamiltonian dependence on injection location and CEP phase and numerically demonstrate that our criterion can be used to determine the onset of electron injection into the bubble.

In the absence of transverse oscillation, Eqns. (2) in main text reduce to

$$\frac{dp_x}{dt} = -\frac{(1+v_b)\xi}{4} + \frac{v_z z}{4}, \frac{dp_z}{dt} = -\frac{(v_x+1)z}{4}, \frac{d\xi}{dt} = \frac{p_x}{\gamma} - v_b, \frac{dz}{dt} = \frac{p_z}{\gamma} \quad (S1)$$

We assume  $v_b = c$  and re scale momentum as  $p_x = R^2 P_x, p_z = R^2 P_z$ , coordinates as  $\xi = XR, z = ZR$ , and time as  $t = Rs$ . Neglecting terms of order  $O(R^{-4}\gamma_b^{-2})$ , the rescaled equations of motion are:

$$\frac{dP_x}{ds} = \frac{X}{2} + \frac{P_z}{\sqrt{P_x^2 + P_z^2}} \frac{z}{4}, \frac{dP_z}{ds} = -\left(1 + \frac{P_x}{\sqrt{P_x^2 + P_z^2}}\right) \frac{Z}{4}, \frac{dX}{ds} = \frac{P_x}{\sqrt{P_x^2 + P_z^2}}, \frac{dZ}{ds} = \frac{P_z}{\sqrt{P_x^2 + P_z^2}} \quad (S2)$$

This equation is parameter-free, and can describe any spherical bubble. Using the initial condition  $P_x = P_z = 0, dP_z/ds = -1/4, dP_x/ds = 0$ , and solving numerically,  $|P_z^{max}| \approx 0.14$ , and  $p_z \approx -0.14R^2$ , as shown in Fig S1 (a).

As was stated in the main text, change in Hamiltonian is  $\Delta H = \int \dot{p}_z(t) \dot{z}_{osc}(t) dt$ . Assuming  $T_{CEP} \gg T_{pass}$ ,  $\sin(\phi_{CEP}) = \sin(\pi/2) = 1$  (optimal phase), we can approximate Hamiltonian increment as  $\Delta H^{(1)} \approx -z_u \omega_{CEP} \Delta p^{(0)}$ . Substituting the maximal value of momentum asymmetry  $\Delta p = 0.14R^2$  from the parameter-free bubble equations to  $\Delta p^{(0)}$ , we get a necessary condition for injection,  $z_u > 7/(\omega_{CEP} R^2)$ .

To show the validity of this criterion, we present numerical results. First, we solve equation of motion Eq. (1-2) for a line of particles placed on y-axis entering the bubble [Fig. S1 (b-c)]. While we chose an oscillating bubble in the main text, injection criteria can be used for any bubble transverse motion, provided the evolution time scale is small much smaller compared to time required for electron to pass through the bubble. For simplicity, we consider bubble motion given by

$$z_{osc}(t) = \begin{cases} z_u \cos(\omega_{CEP} t + \phi_{CEP}), & \text{if } \omega_{CEP} t \leq \pi/2 \\ -z_u, & \text{otherwise} \end{cases} \quad (S3)$$

such that after the time-varying bubble displacement for quarter of oscillation, transverse bubble centroid motion and Hamiltonian stops evolving. We seed the electrons on a line such that electrons near bubble's lower edge ( $z_0 = -R$ ) edge enter bubble at  $\phi_{CEP} = \pi/2$ . The bubble parameters are  $R = 5, \gamma_b = 5, T_{CEP} = 35$ , as outlined in the main text, but we vary oscillation amplitude. Two examples of different oscillation amplitude, one below [Fig S1 (b)]  $z_u = 1.4 < 7/(\omega_{CEP} R^2)$  and one above [Fig S1 (c)]  $z_u = 1.6 > 7/(\omega_{CEP} R^2)$  the threshold are shown. It is seen that electron can be injected when oscillation amplitude is larger than the criteria derived.

Next, we show the CEP-dependence of Hamiltonian evolution: we show two trajectories in Fig. 2(a) in the main text and a trajectory that enters the bubble oscillating with  $T_{CEP} = 50$  at  $z_0 = R, \phi_{CEP} = -\pi/2$  [Fig S1 (d)]. Bubble radius and relativistic factors are identical to that used in the above calculation. Hamiltonians of particles entering the bubble at  $\phi_{CEP} = \pi/2, -\pi/2$  both decrease, but only the Hamiltonian for the bubble oscillating with  $T_{CEP} = 35$  decrease below zero near  $t = 15$ , showing that bubble oscillation must be fast enough. [Fig S1 (e)].

Finally, we show electron capture rate as a function of oscillation amplitude. We simulate interaction between an oscillating potential and background of particles as was done in the main text Fig 2(b-c) using the same parameters but vary the oscillation amplitude and count the number of trapped particles. Electron capture ratio increase as the oscillation amplitude approaches the threshold oscillation amplitude [Fig S1 (f)].

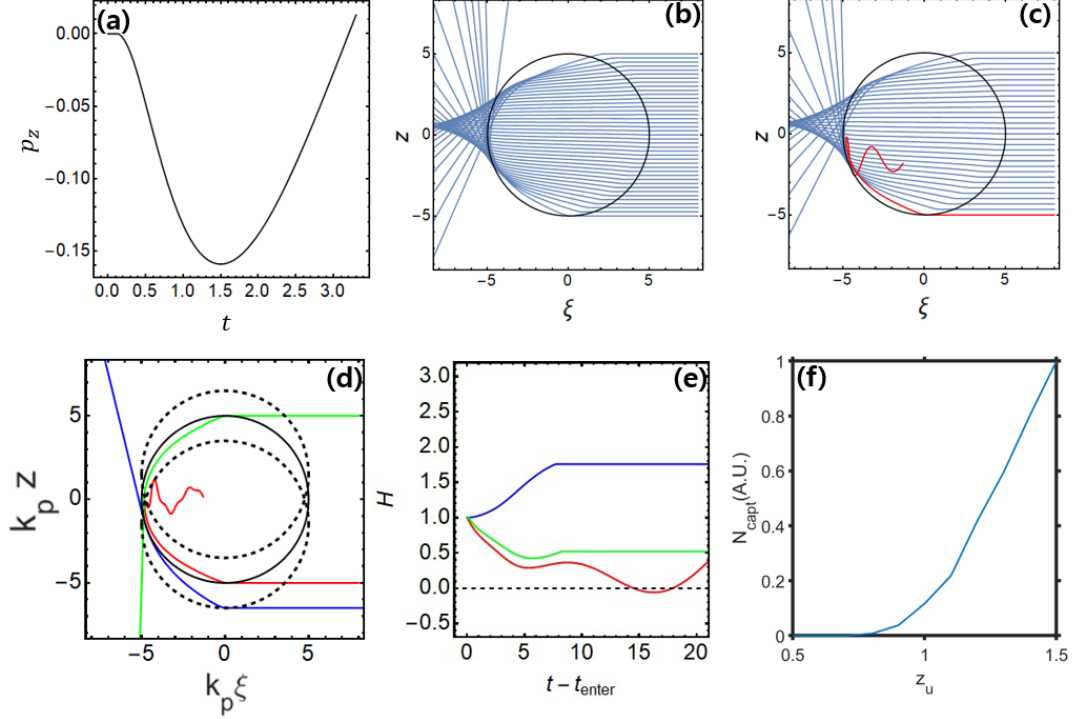

FIG. S1. Demonstration of injection criterion. (a) Normalized Transverse momentum of parameter-free equations. Electron trajectories passing through bubble with oscillation amplitude (b) below ( $z_0 = 1.4$ ) and (c) above ( $z_0 = 1.6$ ) the injection criteria. Untrapped trajectories (light blue line), trapped trajectory (red line), and bubble equilibrium position (black circle). (d-e) Trajectory (d) and evolution of Hamiltonian (e) for two trajectories shown in the main text Fig. 2(a).  $z_0 = -R, \phi_{CEP} = \pi/2, T_{CEP} = 35$  trajectory (Red),  $z_0 = -(R+z_u), \phi_{CEP} = \pi, T_{CEP} = 35$  trajectory (Blue), and  $z_0 = R, \phi_{CEP} = -\pi/2, T_{CEP} = 50$  trajectory (Green). Dashed line in (e) is the  $H = 0$  line. (f) Number of captured particles versus oscillation amplitude.

It should be noted that electrons can enter and leave the bubble at the back while bubble is oscillating. Hence, the trapping criteria may not hold if the bubble has a very high relativistic factor since such bubbles require electrons to gain very high momentum to overtake the bubble. Furthermore, it is also possible that a once trapped particle may exit the bubble due to change in hamiltonian during bubble oscillation. While this complex behavior may seem like a disadvantage, this is also what allows injection of structured electron beam, as explained and demonstrated in the main text.

## II. DISCUSSION ON NON-PONDEROMOTIVE SCALING

CEP effect of a LWFA driven by a single-cycle laser pulse scales as  $\delta p_z \propto a_0^3 \lambda^2 \sin(\phi_{CEP})/\sigma^2 T^2$ , where  $a_0$  is the normalized vector potential,  $\lambda$  is the laser wavelength,  $\phi_{CEP}$  is the laser CEP phase,  $\sigma$  is the laser spot size,  $\sigma_x$  is the longitudinal e-folding length of pulse vector potential envelope, and  $T = \sigma_x/\lambda$  is the cycle number.[2]. In this section, we show that a qualitatively similar scaling holds for the combined fields of a single cycle laser and a trailing non-oscillating bubble using a test particle simulation.

To model asymmetry imparted to plasma by a combination of single-cycle-laser and non-oscillating bubble, we compute momentum/displacement of a swarm of particles on a line  $y_0 = 0, -R < z_0 < R, x_0 = 2R$  after they pass through a single cycle laser and a non-oscillating bubble. The center of single-cycle laser is placed at the front of the bubble,  $x = R$ . We define laser group velocity and bubble velocity in plasma as  $v_g = v_b = \frac{1}{\sqrt{1-\gamma_b^2}}$  with  $\gamma_b = \omega_{inj} = \lambda_p/\lambda_{inj}$  using linear approximation. Laser phase velocity can also be approximated by  $v_{ph} = 1/v_g = 1/v_b$ .

We modify Eqn. S1's momentum equations by adding laser pulse field:

$$\frac{dp_x}{dt} = -\frac{(1+v_b)\xi}{4} + \frac{v_z z}{4} - v_z B_y, \quad \frac{dp_z}{dt} = -\frac{(v_x+1)z}{4} + E_z + v_x B_y \quad (S4)$$

The laser pulse fields are defined as  $E_z = a_0 \omega_{\text{inj}} e^{-(y^2+z^2)/\sigma_{\text{inj}}^2} e^{-(\xi-R)^2/\sigma_x^2} \cos(\omega_{\text{inj}}(x - v_{ph}t - R) + \phi_{CEP})$ ,  $B_y = E_z/v_{ph}$ . The parameters for the bubble and laser field are  $a_0 = 4$ ,  $\sigma_{\text{inj}} = 3$ ,  $R = 5$ .

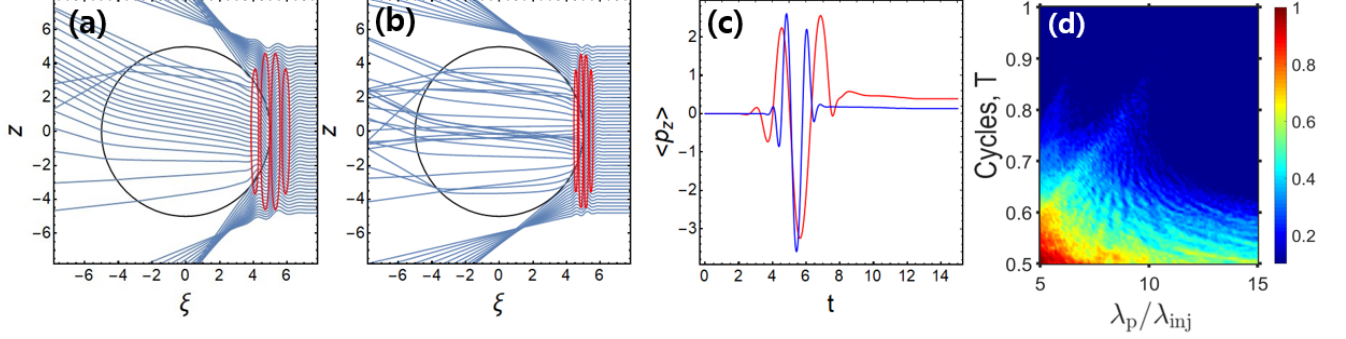

FIG. S2. Asymmetric electron response under combined fields of laser and non-oscillating bubble. (a-b) Electron trajectory deflection under combined fields for  $T = \sigma_x/\lambda_{\text{inj}} = 1$ , (a)  $\lambda_p = 5\lambda_{\text{inj}}$  and (b)  $\lambda_p = 10\lambda_{\text{inj}}$ . Bubble boundary (black),  $a_0 = 1$  contour (red), electron trajectory (blue). (c) Average momentum of electrons over time for  $\lambda_p = 5\lambda_{\text{inj}}$  (blue) and  $\lambda_p = 10\lambda_{\text{inj}}$  (red). (d) Parameter scan computing  $\delta z_{ex}$  over laser wavelength and number of wavelength, as shown in main text.

Electron deflection through the combined fields for  $\phi_{CEP} = \pi/2$  are shown in Fig S2 (a-b). Larger asymmetry of particle trajectories passing through the bubble for longer wavelength pulse is evident. Resulting average momentum  $\langle p_z \rangle$  over time is shown in Fig S2(c), confirming larger asymmetry for longer wavelength pulse.

To quantify asymmetry over parameter space, a parameter scan computing average transverse displacement  $\delta z_{ex} = \langle z_{ex} \rangle$  was carried out over cycle number ( $T = \sigma_x/\lambda_{\text{inj}}$ ) and ratio between laser wavelength. To reduce the effect of CEP phase and simply extract the magnitude of asymmetry, particles were seeded on range  $2R < x_0 < 2R + v_g T_{CEP}$ ,  $y_0 = 0$ ,  $-R < z_0 < R$  such that they would sample one CEP period of the laser. Each particle is removed from the simulation after reaching the end of the bubble at the exit time  $t_{\text{ex}}$  such that  $\xi(t_{\text{ex}}) = -R$ , and its transverse displacement  $z_{\text{ex}} = z(t_{\text{ex}})$  is recorded upon exit. This computation shows that asymmetry grows as the cycle number decreases and the injector pulse wavelength increases [Fig S2 (d)].

When laser spot size  $\sigma_{\text{inj}}$  and ponderomotive potential  $U_p \propto P_{\text{inj}} \lambda_{\text{inj}}^2 / \sigma_{\text{inj}}^2 \propto a_0^2$  are kept constant, momentum asymmetry  $\delta p_z \propto U_p^{3/2} \lambda_{\text{inj}}^2 / \sigma_{\text{inj}}^2$  can be increased by using longer wavelength injector pulse. Furthermore, because we fix the ponderomotive potential, smaller power pulse is required to get comparable asymmetry. These two advantages are exploited and reflected on the PIC simulations of the main text.

### III. EFFECT OF CHANGING INJECTOR PULSE

In the main text, we use several different CEP pulses and show that they result in different bunch profile. In this section, we show that the bunch profile can be modified using different injector pulses and that, in case of a circularly polarized injector, we can get continuous injection resulting in disappearance of current spikes. Furthermore, we show that terminating plasma and observing one of the bunches' deflection can be a direct observable for kicker CEP from experiments.

#### A. Circularly polarized injector pulse

While we consider a linearly polarized pulse in the main text, near-single-cycle circularly polarized pulses have also been generated recently [3]. The consequence of using such pulses for injection results in a drastically different injected bunch profile.

Instead of a transversely oscillating bubble, we now consider a bubble whose centroid executes a spiral motion defined as  $r(\vec{t}) = r_u \{ \hat{z} \sin(\omega_{CEP}t + \phi_{CEP}) + \hat{y} \cos(\omega_{CEP}t + \phi_{CEP}) \} = \hat{z} z_{osc}(t) + \hat{y} y_{osc}(t)$ . Now equations of motion in all three dimensions must be considered.

$$\frac{dp_x}{dt} = -\frac{(1+v_b)\xi}{4} + \frac{v_y \tilde{y}(t)}{4} + \frac{v_z \tilde{z}(t)}{4} - \frac{\tilde{y}(t) \dot{y}_{osc}(t)}{4} - \frac{\tilde{z}(t) \dot{z}_{osc}(t)}{4}, \quad \frac{dp_y}{dt} = -\frac{(v_x+1)\tilde{y}(t)}{4}, \quad \frac{dp_z}{dt} = -\frac{(v_x+1)\tilde{z}(t)}{4} \quad (\text{S4})$$

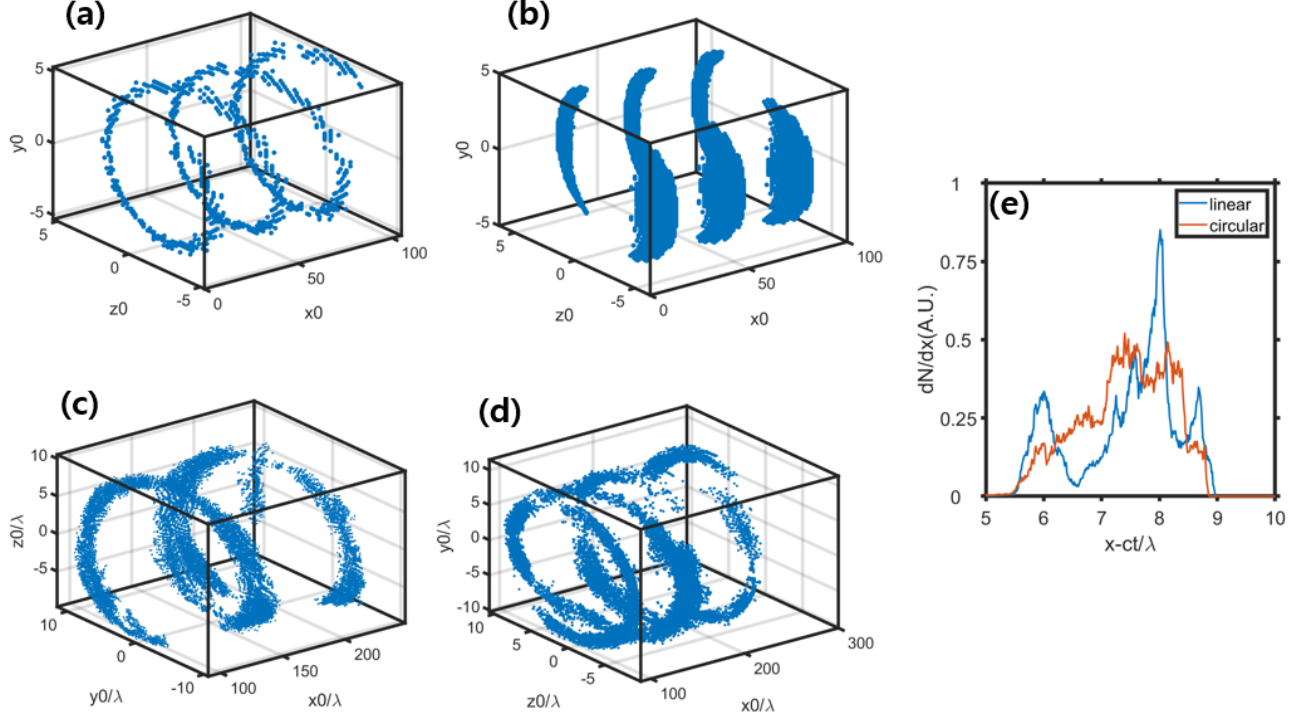

FIG. S3. Control of longitudinal bunching via injector pulse polarization. (a-d) Initial position of trapped electrons from test-particle simulations(a-b) and PIC simulations(c-d). Panels (a,c) show results for circularly polarized injector pulse and (b,d) show results for linearly polarized injector pulse. (e) Longitudinal profile of injected bunches from PIC simulation. Coordinates of (a-b) are normalized to  $k_p^{-1}$

with  $\tilde{y}(t) = y - y_{osc}(t)$ ,  $\tilde{z}(t) = z - z_{osc}(t)$ .

Unlike the CEP effect in one direction which has optimal phases for injection, this bubble formed by a circularly polarized pulse can always inject electrons because bubble center is rotating and has a finite displacement/velocity at all times. This leads to continuous injection from background plasma, originating from a spiral-shaped initial position.

A result from a test particle simulation and PIC simulation similar to that used for the Fig 2(c-d) in the main text ( $R = 5$ ,  $z_u/R = 0.4$ ,  $r_u/R = 0.4$ ,  $T_{CEP} = 35$ ,  $\gamma_b = 5$ ) with a bubble formed by circularly polarized pulse shows that injected electrons indeed originate from a spiral location. Initial positions of injected particles trapped by bubble formed by a circularly polarized pulse and linearly polarized pulse are plotted in Fig S3(a-b), and the corresponding PIC results are plotted in Fig S3 (c-d). The resulting longitudinal current in the PIC simulation S3 (e) has less modulation in the circularly-polarized case.

## B. Control of Bunch transverse structure via CEP

Because injector pulse has dominant effect on injection process via CEP effect, altering its initial CEP can alter the transverse structure of the injected bunch. Change in injector CEP phase leads to different injected bunch profiles, as shown in Fig S4 (a-c). Furthermore, changing the CEP phase by  $\pi$  results in a bunch profile [Fig S4(c)] that is a mirror image of  $\phi_{CEP} = 0$  [Fig S4(a)].

Measuring one of the bunch deflection angle after terminating the plasma can yield an observable for CEP effect. We plot three pictures of the CEP-injected bunches after plasma termination [S4 (d-f)]. By measuring the deflection of one of the beam, for instance the one at  $x - ct/\lambda = 8.5$ , one may retrieve CEP of the injector pulse.

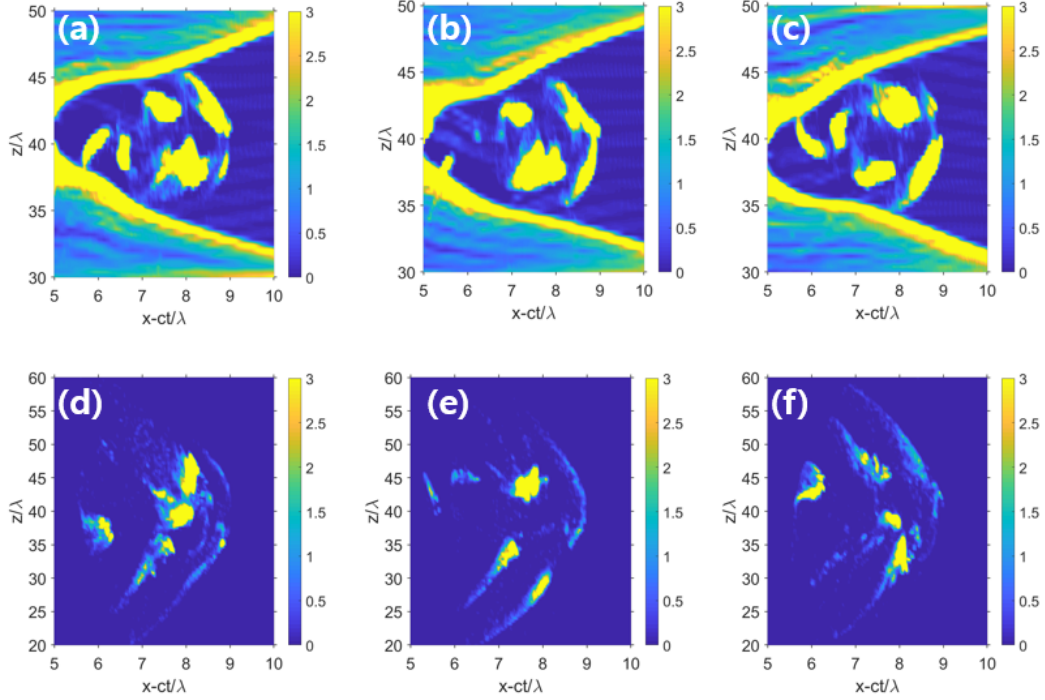

FIG. S4. Transverse profile control via injector pulse phase change. (a-c) Injected bunch distribution in x-z plane for  $x = 0.28\text{mm}$  propagation. (d-f) Injected bunch distribution in x-z plane for  $x = 0.56\text{mm}$  propagation after plasma termination at  $x = 0.4\text{mm}$ .  $\phi_{CEP} = 0$ (a,d),  $\phi_{CEP} = \pi/2$ (b,e),  $\phi_{CEP} = \pi$ (c,f)

#### IV. DIFFERENCE IN TIME SCALE BETWEEN THE INJECTOR AND DRIVER PULSE

One of the key features of the two-pulse scheme utilized in the main text is the difference in pulse evolution time-scale. Laser depletion distance is proportional to  $L_{\text{etch}} \propto \lambda_L^2/\lambda_p^2$ .  $\lambda_{\text{inj}} = 3\lambda_{\text{dr}}$  [4], so ratio between the depletion distances for driver ( $L_{\text{dr}}$ ) and injector pulse ( $L_{\text{inj}}$ ) is  $L_{\text{inj}}/L_{\text{dr}} \approx 9$ . This is evidenced by the very quick decay of peak amplitude of injector pulse, compared to a much slower decay of pump pulse peak amplitude [Fig S5]. Because of this discrepancy in depletion time, injector pulse generates a relatively short injection region, after which injection is terminated and stable acceleration follows.

This time-scale difference is crucial for a relatively low-emittance, low-energy spread beam. If the cavity keeps oscillating, electrons will continuously get injected, resulting in a much longer train of beam. Furthermore, the cavity oscillation will modify the already injected and relativistic beam for a long time. These effects can compromise beam quality significantly. By using this evolution time-scale difference between the two pulse, we can get localized injection and can curtail such adverse effects.

#### V. OVERALL EMITTANCE OF WHOLE BEAM VERSUS OVERALL EMITTANCE OF INDIVIDUAL BEAM

In our injection scheme, there are multiple injections. We show that these injected electrons form a coherent bunch instead of a cloud of incoherent electrons by calculating the emittance of one of the bunches. Emittance of the electrons located at  $x - ct/\lambda \approx 9$  in the range of  $|\gamma - 680| < 35$  is  $\epsilon_{\perp} = \sqrt{(\langle r^2 \rangle \langle p_r^2 \rangle - \langle r p_r \rangle^2)} \approx 0.94\text{mm} \pi$  mrad. Without subtracting the  $\langle r p_r \rangle^2$  term, the emittance is  $2.62\text{mm} \pi$  mrad. Subtraction of this cross-product term would not reduce the emittance if the electrons were undergoing incoherent motion. This shows that injected bunches undergo significant transverse oscillations in a coherent manner, and should be considered as individual relatively low-emittance beams.



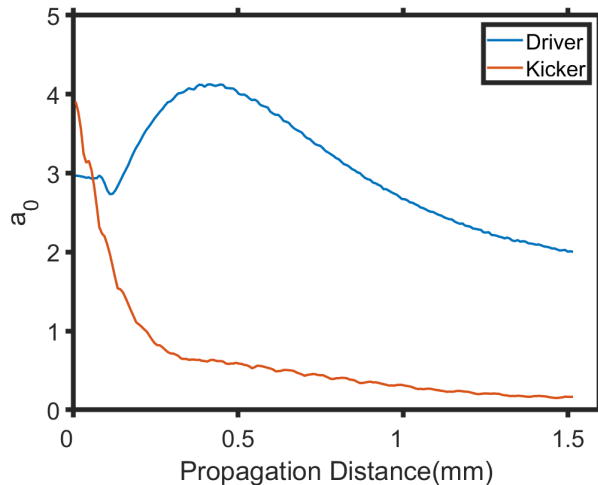

FIG. S5. Peak normalized field strength of Driver and injector pulse.

## VI. CONFIRMATION OF NECESSITY OF OSCILLATION FOR INJECTION USING 2D SIMULATION

In the main text, we have shown that transverse oscillation of an oscillating plasma bubble can trap electrons. To further confirm that such oscillation is necessary for injection, we ran 2D PIC simulations where electron response in the p-plane and s-plane can be decoupled. CEP effect induces oscillation in the laser polarization direction. This means that if the injector is s-polarized, a transversely symmetric response can be generated in 2D. We can compare this result with the p-polarized injector result, and ascertain that presence(absence) of oscillation indeed triggers the injection on(off).

We run two 2D simulations, each using two linearly polarized pulses separated by  $\Delta T = 37\text{fs}$  launched into plasma identical to that used in the main text. For both simulations, driver pulse trailing behind is s-polarized, and long wavelength injector pulse polarization is varied, one p-polarized and one s-polarized. Pulse parameters are given in Table S1. The parameters are different from those in the main text due to difference between 2D and 3D simulations.

TABLE S1. Pulses' Parameters for 2D Simulation

| Laser pulse  | Driver                                 | Injector                                |
|--------------|----------------------------------------|-----------------------------------------|
| Polarization | y                                      | z or y                                  |
| Wavelength   | $\lambda_{\text{dr}} = 0.8\mu\text{m}$ | $\lambda_{\text{inj}} = 3.2\mu\text{m}$ |
| FWHM         | $T_{\text{dr}} = 22\text{fs}$          | $T_{\text{inj}} = 8\text{fs}$           |
| Spot Size    | $\sigma_{\text{dr}} = 8\mu\text{m}$    | $\sigma_{\text{inj}} = 6\mu\text{m}$    |
| Peak power   | $P_{\text{dr}} = 31\text{TW}$          | $P_{\text{inj}} = 2.4\text{TW}$         |

Indeed, it is seen that only the p-polarized injector can inject electrons into the plasma bubble [Fig S6]. Furthermore, difference in time scale between the injector and driver pulse is also observed: the plasma bubble is almost symmetric at  $x = 0.8\text{mm}$  propagation, showing that injector pulse indeed decays very quickly and has negligible role played in the later acceleration process. However, the injected electrons in the p-polarized injector simulation [Fig S6 (a)] shows that the injected electrons are distributed asymmetrically, carrying information from their asymmetric injection process.

## VII. SIMULATION DETAILS

The 2D/3D PIC simulations were performed using the PIC code VLPL[5]. Simulation box with a moving window of  $x \times y \times z = 40\mu\text{m} \times 64\mu\text{m} \times 64\mu\text{m}$  with  $\Delta x \times \Delta y \times \Delta z = \lambda_{\text{dr}}/25 \times \lambda_p/50 \times \lambda_p/50$  with 4 particles per cell was used for 3D simulation. Simulation box with  $x \times y = 40\mu\text{m} \times 80\mu\text{m}$  with  $\Delta x \times \Delta y = \lambda_{\text{dr}}/25 \times \lambda_p/50$  with 8 particles per cell was used for 2D simulations. Lasers pulses were focused to the edge of plasma with a  $0.03\text{mm}$  upramp, leading

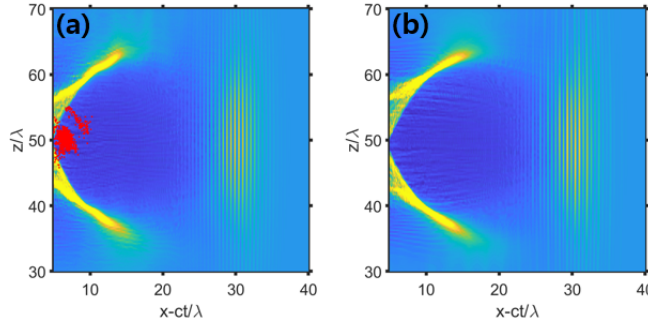

FIG. S6. 2D simulation results. Density for p-polarized (a) and s-polarized(b) injector pulse (colormap) and injected electrons(red dots) at propagation distance  $0.8mm$

to plateau density of  $4.4 \times 10^{18}/cm^3$

- 
- [1] I. Yu. Kostyukov, E. N. Nerush, A. Pukhov, and V. Seredov, “Electron Self-Injection in Multidimensional Relativistic-Plasma Wake Fields,” *Phys. Rev. Lett.*, **103**, 175003 (2009).
  - [2] E.N. Nerush, and I. Yu. Kostyukov, “Carrier-Envelope Phase Effects in Plasma-Based Electron Acceleration with Few-Cycle Laser Pulses,” *Phys. Rev. Lett.*, **103**, 035001 (2009).
  - [3] F. Salehi , M. Le , L. Railing, and H. M. Milchberg, “Laser-accelerated, low divergence 15 MeV quasi-monoenergetic electron bunches at 1 kHz”, *arXiv* 2010.15720,(2020)
  - [4] W. Lu, M. Tzoufras, C. Joshi, F.S. Tsung, W.B. Mori, J.Vieira, R. Fonseca, and L.O.Silva, “Generating multi-GeV electron bunches using single stage laser wakefield acceleration in a 3D nonlinear regime,” *Phys. Rev. ST Accel. Beams*, **10**, 061301 (2007).
  - [5] A. Pukhov, “Three-dimensional electromagnetic relativistic particle-in-cell code VLPL (Virtual Laser Plasma Lab),” *J. Plasma Phys.* **61**, 425 (1999).
